# Supplementary material for: Self-supervised Transparent Liquid Segmentation for Robotic Pouring
Source: arXiv:2203.01538 source file (2022-03-03)
Supplement: Supplementary file 1 [file 7-appendix.tex]

% CUT architecture details

% Background Subtraction
%     Colored Liquids
%     Transparent Liquids (failure case)

% Segmentation Network architecture

% Vision system
%     data capture
%     frequency
%     Height detection
